# Supplementary material for: Governing Strategic Dynamics: Equilibrium Stabilization via Divergence-Driven Control
Source: arXiv:2506.23734 ancillary file (2026-01-28)
Supplement: Supplementary file 1 [file supplementary.pdf]

# Supplementary Material for

## Marker Gene Method : Identifying Stable Solutions in a Dynamic Environment

Hao Shi, Xi Li, Fangfang Xie

---

### I. Proof of MGM Convergence and Stability

This section provides the detailed mathematical proofs for the convergence and stability properties of the Marker Gene Method (MGM) presented in the main paper.

#### A. Notations and Problem Setup

We begin by defining the key notations and the game-theoretic setting used throughout the proofs.

##### 1) Game Theoretic Setting:

- $G = (S_1, S_2, u_1, u_2)$ : A two-player game, assumed to be a Strictly Competitive Game (SCG).
- $S_1, S_2$ : Pure strategy sets for player 1 and player 2, respectively.
- $u_1 : S_1 \times S_2 \rightarrow \mathbb{R}, u_2 : S_1 \times S_2 \rightarrow \mathbb{R}$ : Payoff functions for player 1 and player 2.
- $d_1 = |S_1|, d_2 = |S_2|$ : The number of pure strategies for player 1 and player 2. For simplicity in some derivations, we may assume  $d_1 = d_2 = d$ .
- $p \in \Delta^{d_1-1}, q \in \Delta^{d_2-1}$ : Mixed strategies for player 1 and player 2, where  $\Delta^{k-1}$  is the  $(k-1)$ -dimensional probability simplex.
- $A$ : Payoff matrix for player 1 (rows are player 1's strategies, columns are player 2's strategies). Expected payoff for player 1 is  $p^\top A q$ .
- For SCGs, the game can be transformed into an equivalent zero-sum game with payoff matrix  $R$  for player 1, where  $R = -R^\top$  (antisymmetric) after normalization, and player 2's payoff is  $-p^\top R q$ .
- $p_C$ : Latent variable strategy (e.g., marker gene strategy from the opposing population), sampled according to a distribution  $\mu$ . Often assumed to be  $p_C \sim \text{Dirichlet}(1, \dots, 1)$  (uniform on the simplex) representing maximum uncertainty or an exploratory opponent.

##### 2) MGM Specific Notations: Let $i$ and $j$ be indices for individuals (strategies) within a population.

- $M_i = u_1(p_i, p_C)$ : Marker Gene Fitness of individual  $i$  (strategy  $p_i$ ) against the current marker gene strategy  $p_C$ . This is a single encounter score.
- $G_i = \frac{1}{n_{eval}} \sum_{k=1}^{n_{eval}} u_1(p_i, q_k)$ : Generalization Fitness of individual  $i$  (strategy  $p_i$ ) averaged over  $n_{eval}$  encounters with opponents  $q_k$  sampled from the opposing population (or a test set).
- $\omega$ : Base weight parameter for combining  $M_i$  and  $G_i$ .
  - $\omega_0 = \omega$ : Fixed baseline weight, typically  $w_0 = 0.9$ .
  - $\omega_i = w(G_i, M_i)$ : Dynamic weight for individual  $i$ , a function of its  $G_i$  and  $M_i$ . Typically  $w_i \leq w_0$ .
- $F_i$ : Total Fitness of individual  $i$ .
  - For fixed-weight individuals (or as a baseline):  $F_i := w_0 M_i + (1 - w_0) G_i$ .
  - For dynamic-weight individuals:  $F_i := w_i M_i + (1 - w_i) G_i$ .
- $\Delta M_{ij} := M_i - M_j$ : Difference in marker gene fitness.
- $\Delta G_{ij} := G_i - G_j$ : Difference in generalization fitness.

- $\mathcal{E}_1$ : Ranking Reversal Event for fixed-weight individuals, defined as  $\{\Delta M_{ij} > 0 \text{ and } F_j > F_i \text{ when } w_i = w_j = w_0\}$ .
  - $\eta = w_0/(1 - w_0)$ .
  - $G_0 = \eta \Delta M_{ij}$ .
- $\mathcal{E}_2$ : Ranking Reversal Event for dynamic-weight individuals
- $\mathcal{E}_3$ : Ranking Reversal Event involving dynamic-weight individuals (cross-set ranking).
- $\mathcal{E}$ : General marker gene update event where an old marker gene is replaced by a new one.
- $l$ : Target fitness threshold (e.g., slightly below NE payoff) for marker gene update mechanism.
- $F(i, t)$ : The individual  $i$  when it is in generation  $t$ .
- $K$ : KeepCount/BufferCount; number of consecutive generations a condition must hold for marker gene update.
- $N_{pop}$ : Population size.
- $k$ : The number of an individual evaluation games.
- $p^*$ : A Nash Equilibrium strategy.
- $\mathcal{N}_\epsilon(p^*)$ : An  $\epsilon$ -neighborhood of the Nash Equilibrium  $p^*$ .
- $L = \text{Lip}(h \circ g_1)$ : Lipschitz constant of the transformation from original payoff  $u_1$  to the normalized antisymmetric payoff  $R$ .
- $\phi(i, C) := p_i^\top R p_C^\top$ : Transformed one-shot game score.
- $\Sigma = R \cdot \mathbb{E}[p_C p_C^\top] \cdot R^\top$ : Core covariance matrix component.
- $\rho_M, \rho_G$ : Correlation coefficients for  $M_i, M_j$  and  $G_i, G_j$  respectively.
- $\alpha$ : Small noise intensity in SDE models, typically  $\alpha = \mathcal{O}(1/\sqrt{N_{pop}})$ .
- $\alpha(x)$ : Dynamic adjust weight function.
- $\beta$ : The difference of base fitness and  $l$ .
- $V(x)$ : Quasi-potential function in Freidlin-Wentzell theory.
- $\tau_{escape}$ : Mean escape time from an attractor.
- $f_i(x)$ : Drift term for strategy  $i$  in the replicator dynamics ODE.
- $\Phi(x)$ : Average fitness of the population  $\sum_k x_k f_k(x)$ .
- $J(x^*)$ : Jacobian matrix of the ODE system at  $x^*$ .
- $\text{div} f(x^*)$ : Divergence of the vector field  $f$  at  $x^*$ .
- $\text{Var}(X)$ : The variance of  $X$ .

## B. Key Assumptions Underpinning the Proofs

Assumption B.1 (M Distribution (Baseline Fitness)). For any individual  $s$ , its baseline fitness  $M_s$  is drawn from a distribution on  $[0, C_M]$ . The probability density function (PDF) of  $M_s$ , denoted by  $f_M(m)$ , is bounded, i.e.,  $f_M(m) \leq C_M^{pdf}$  for some constant  $C_M^{pdf} > 0$ . The baseline fitness values  $M_s$  for different individuals  $s$  are approximately independent and identically distributed (i.i.d.).

Assumption B.2 (G Generation (Generalization Fitness)). The generalization fitness  $G_s$  for an individual  $s$  is computed as the average of  $n_{eval}$  independent evaluations against opponents randomly drawn from the opposing population. Specifically,  $G_s = \frac{1}{n_{eval}} \sum_{r=1}^{n_{eval}} X_{s,r}$ , where each  $X_{s,r} \in [0, C_G]$  is the outcome of the  $r$ -th evaluation. For simplicity in some analyses, we may consider  $C_G = 1$ .

Assumption B.3 (Independence of (M,G) Pairs). For any two distinct individuals  $s$  and  $t$ , the pair of fitness values  $(M_s, G_s)$  is approximately independent of the pair  $(M_t, G_t)$ . Furthermore, within an individual  $s$ ,  $M_s$  and  $G_s$  are treated as approximately independent for analytical tractability, though they may exhibit correlations in practice.

Assumption B.4 (Nash Equilibrium Properties). Let  $x^* = (x_1^*, x_2^*) \in \Delta_1 \times \Delta_2$  be a strictly mixed Nash Equilibrium (NE) of the underlying game  $G = (S_1, S_2, u_1, u_2)$ . The expected payoff functions for player  $k$ ,  $u_k(p, q)$  where  $p \in \Delta_1, q \in \Delta_2$ , are assumed to be twice continuously differentiable ( $C^2$ ) with respect to their arguments in the simplex, and  $x^*$  is an interior point of  $\Delta_1 \times \Delta_2$ .

Assumption B.5. The single-round payoff  $R_{ij} \in [-1, 1]$  is bounded, and payoffs across different rounds are independent.

Assumption B.6. In each generation, each individual is randomly matched  $k$  times, where  $c_1 > 0$  is a constant.

Assumption B.7. Two independent sample batches are used for evaluating old/new marker genes.

### C. Weak Correlation Analysis in Strictly Competitive Games (SCGs)

Rationality Analysis of the Approximate Independence Assumption for  $(M_i, G_i)$  and  $(M_j, G_j)$  (B.3) and the Assumption that  $M_k, G_k \sim \text{i.i.d. on } [\mathcal{A}, \mathcal{B}]$  (B.1, B.2): We note that, strictly speaking, when  $M_i$  and  $M_j$  are evaluated against the same opponent population (or individual), a common latent variable  $C$  (representing the opponent's strategy or state) is introduced, leading to statistical dependence between  $M_i$  and  $M_j$ . Similarly, since  $G_i$  and  $G_j$  are also evaluated against the same (opponent NE strategy or population used for generalization assessment),  $G_i$  and  $G_j$  will also exhibit statistical dependence.

While we acknowledge this inherent statistical dependence in MGM, analyzing co-evolutionary systems under such complete dependence is often intractable, as it requires complex modeling of the joint distributions involved. Considering the inherent characteristics of many co-evolutionary systems, this dependence is often significantly weakened:

- 1) **Intransitivity and Complex Interactions:** Co-evolutionary processes often exhibit intransitive relationships (e.g., Rock-Paper-Scissors dynamics), and the actual fitness calculation depends on complex combinations of strategies. This makes it difficult to directly predict the outcome of individual  $C$  against individual  $B$  by observing the outcome of individual  $A$  against individual  $B$ . Therefore, the ability to infer  $M_j$ ,  $G_i$ , and  $G_j$  by observing  $M_i$  is very limited, or even unpredictable. For instance, in the RPS game, due to the strategic dominance cycle, it is impossible to infer  $M_j$  from  $M_i$  without observing the strategy of  $B$ .
- 2) **High-Dimensional Strategy Spaces and Genotypic Complexity:** When strategies have complex genotypes and intricate fitness function mappings, even genotypically similar individuals can exhibit vastly different scalar fitness values upon evaluation. This chaotic behavior tends to reduce the statistical dependence introduced by using common evaluation criteria.
- 3) **Randomness and Averaging Effects:** The inherent randomness of evolutionary operators and potentially the evaluation process itself contribute significant noise. Considering the law of large numbers, for generalization fitnesses  $G_i$  and  $G_j$  (which are often averages over multiple evaluations), the dependence-weakening effect of this noise is further amplified by averaging.

Therefore, in co-evolutionary systems, we consider approximating this statistical dependence as independence, making the assumption:  $(M_i, G_i)$  and  $(M_j, G_j)$  are approximately independent for  $i \neq j$ . This assumption allows the overall co-evolutionary system to be analyzed using standard probabilistic tools. Specifically, this assumption permits the use of Hoeffding's inequality to bound the deviation of generalization fitness and allows us to analyze the contribution of dynamic weights using techniques that rely on joint probability factorization or the application of union bounds under independence. This facilitates the derivation of analytical relationships between event probabilities  $P(E)$  and key system parameters (such as the generalization evaluation sample size  $n$ ).

We acknowledge that this assumption is a simplification of the underlying system. Although we have argued for its reasonableness based on the inherent complexities of co-evolutionary systems, we cannot entirely rule out the impact of this assumption on the actual derived results.

**Definition C.1 (Strictly Competitive Game Property).** For all strategy pairs  $(s_1, s_2), (s_1^*, s_2^*) \in S_1 \times S_2$ , the following holds:

$$u_1(s_1, s_2) > u_1(s_1^*, s_2^*) \iff u_2(s_1, s_2) < u_2(s_1^*, s_2^*). \quad (\text{I.1})$$

Lemma C.2 (Transformation to Zero-Sum Game). There exist strictly monotonically increasing functions  $g_1, g_2$  such that the transformed utilities  $u'_1 = g_1(u_1)$  and  $u'_2 = g_2(u_2)$  satisfy:

$$u'_1 + u'_2 \equiv 0 \quad (\text{I.2})$$

This transformed zero-sum game shares the same Nash Equilibria (NE) and preference orderings as the original SCG.

Lemma C.3 (Transformation to Anti-Symmetric Payoff Matrix). Define the payoff matrix  $\mathbf{R}'$  for the zero-sum game, with elements:

$$R'_{AB} = u'_1(A, B) \quad (\text{I.3})$$

A common strictly increasing function  $h$  (possibly the identity function) can be found such that the final payoff matrix :

$$\mathbf{R} = h(\mathbf{R}') \quad (\text{I.4})$$

satisfies anti-symmetry.

$$\mathbf{R} = -\mathbf{R}^\top \quad (\text{I.5})$$

and can be normalized such that

$$\max_{A,B} |R_{AB}| \leq 1 \quad (\text{I.6})$$

Anti-symmetry ensures that  $\mathbf{R}\mathbf{1} = \mathbf{0}$  (row sums and column sums are zero, where  $\mathbf{1}$  is a vector of ones).

Definition C.4 (Lipschitz Constant). Let:

$$L = \text{Lip}(h \circ g_1) \quad (\text{I.7})$$

be the Lipschitz constant of the entire transformation process from the original payoff  $u_1$  to the final normalized anti-symmetric payoff  $R_{AB}$ .

1) Deriving Covariance Bounds using Anti-symmetric Structure and High-Dimensional Effects:

Proposition C.5 (Single Bout Score). The score of a single encounter (after transformation) is :

$$\phi(i, C) := \mathbf{p}_i^\top \mathbf{R} \mathbf{p}_C \quad (\text{I.8})$$

where  $\mathbf{p}_i$  is the one-hot encoding of player 1's pure strategy  $i$ , and  $\mathbf{p}_C$  is the mixed strategy of the opponent (player 2).

Lemma C.6 (Covariance Core Term). We are primarily interested in  $|\mathbb{E}[\phi(i, C)\phi(j, C)]|$  (assuming mean is close to 0 or data is centered):

$$|\mathbb{E}[\phi(i, C)\phi(j, C)]| = |\mathbb{E}[(\mathbf{p}_i^\top \mathbf{R} \mathbf{p}_C)(\mathbf{p}_j^\top \mathbf{R} \mathbf{p}_C)]| \quad (\text{I.9})$$

$$= |\mathbf{p}_i^\top \mathbf{R} \mathbb{E}[\mathbf{p}_C \mathbf{p}_C^\top] \mathbf{R}^\top \mathbf{p}_j| \quad (\text{I.10})$$

Lemma C.7 (Second Moment Matrix). Let

$$\Sigma_{\text{payoff}} = \mathbf{R} \mathbb{E}[\mathbf{p}_C \mathbf{p}_C^\top] \mathbf{R}^\top \quad (\text{I.11})$$

When  $\mathbf{p}_C \sim \text{Dirichlet}(\mathbf{1}_d)$  (i.e., Dirichlet distribution with all concentration parameters equal to 1, over  $d$  opponent pure strategies), then :

$$\mathbb{E}[\mathbf{p}_C \mathbf{p}_C^\top] = \alpha \mathbf{I} + \beta \mathbf{J} \quad (\text{I.12})$$

where  $\alpha = \frac{1}{d(d+1)}$ ,  $\beta = \frac{1}{d(d+1)}$ , and  $\mathbf{J} = \mathbf{1}\mathbf{1}^\top$  is the matrix of all ones. Since  $\mathbf{R}\mathbf{1} = \mathbf{0}$  (from Lemma C.3), it implies  $\mathbf{R}\mathbf{J} = \mathbf{0}$  and  $\mathbf{J}\mathbf{R}^\top = \mathbf{0}$ . Therefore:

$$\Sigma_{\text{payoff}} = \mathbf{R}(\alpha \mathbf{I} + \beta \mathbf{J}) \mathbf{R}^\top = \alpha \mathbf{R} \mathbf{R}^\top. \quad (\text{I.13})$$

Lemma C.8 (Spectral Norm Bound ). We need to bound  $\|\Sigma_{\text{payoff}}\|_2 = \alpha \lambda_{\max}(\mathbf{R} \mathbf{R}^\top)$ . Consider the following cases:

a) Case 1.1: Special Structure (e.g., Cyclic / Fully Ordered): Many important benchmark games (like generalized RPS) satisfy the structure:

$$R_{ij} = \text{sign}(\pi(j) - \pi(i)) \quad (\star)$$

where  $\pi$  is a permutation.

Lemma C.9 (For Special Structure  $(\star)$ ). For a matrix  $\mathbf{R}$  satisfying structure  $(\star)$ , it can be rigorously proven that

$$\mathbf{R}\mathbf{R}^\top = d\mathbf{I} - \mathbf{J} \quad (\text{I.14})$$

.The spectrum of this matrix is  $\{0 \text{ (multiplicity } 1), d \text{ (multiplicity } d-1)\}$ .

Corollary C.10 ( $\lambda_{\max}$  for Special Structure ).  $\lambda_{\max}(\mathbf{R}\mathbf{R}^\top) = d$ .

Substituting to calculate  $\|\Sigma_{\text{payoff}}\|_2$ :

$$\|\Sigma_{\text{payoff}}\|_2 = \alpha \lambda_{\max}(\mathbf{R}\mathbf{R}^\top) = \frac{1}{d(d+1)} \cdot d = \frac{1}{d+1} = O\left(\frac{1}{d}\right). \quad (\text{I.15})$$

At this point, the covariance bound is:

$$|\text{Cov}(M_i, M_j)| \approx |\mathbf{p}_i^\top \Sigma_{\text{payoff}} \mathbf{p}_j| \quad (\text{I.16})$$

$$\leq L^2 \cdot \|\mathbf{p}_i\|_2 \|\mathbf{p}_j\|_2 \cdot \|\Sigma_{\text{payoff}}\|_2 \quad (\text{I.17})$$

$$\leq L^2 \cdot 1 \cdot 1 \cdot O\left(\frac{1}{d}\right) \quad (\text{assuming } M_i, M_j \text{ are based on transformed } R)$$

$$= O\left(\frac{L^2}{d}\right) \quad (\text{I.18})$$

Here, we use  $L^2$  to convert back to the original payoff scale, conservatively estimating  $\|\mathbf{p}\|_2 \leq 1$  for general mixed strategies, though for pure strategies  $\|\mathbf{p}_i\|_2 = 1$ .

Therefore, the correlation coefficient

$$\rho_M = O\left(\frac{L^2}{d}\right) \quad (\text{I.19})$$

b) Case 2.2: General Anti-symmetric SCG (No Special Structure): If we do not assume structure  $(\star)$ , we only know  $\mathbf{R} = -\mathbf{R}^\top$ ,  $|R_{ij}| \leq 1$ , and  $\mathbf{R}\mathbf{1} = \mathbf{0}$ .

Lemma C.11 (Trace Inequality for  $\lambda_{\max}$  ). Using a strict trace inequality:

$$\lambda_{\max}(\mathbf{R}\mathbf{R}^\top) \leq \text{tr}(\mathbf{R}\mathbf{R}^\top) = \sum_i \|\mathbf{r}_i\|_2^2 \leq d(d-1) \quad (\text{I.20})$$

Substituting to calculate  $\|\Sigma_{\text{payoff}}\|_2$ :

$$\|\Sigma_{\text{payoff}}\|_2 = \alpha \lambda_{\max}(\mathbf{R}\mathbf{R}^\top) \quad (\text{I.21})$$

$$\leq \frac{1}{d(d+1)} \cdot d(d-1) = \frac{d-1}{d+1} = O(1). \quad (\text{I.22})$$

In this case,  $\|\Sigma_{\text{payoff}}\|_2$  no longer decays with  $d$ . However, in many high-dimensional scenarios or regions near NE, the deviation  $\boldsymbol{\delta} = \mathbf{p} - \mathbf{p}^*$  of a strategy  $\mathbf{p}$  from NE ( $\mathbf{p}^*$ ) typically scales with increasing dimension, i.e.,  $\|\boldsymbol{\delta}\| = \Theta(1/\sqrt{d})$  or  $O(1/\sqrt{d})$ .

Assumption C.12 (Scaling of Strategy Distribution Deviation ). The deviation of strategy distributions satisfies  $\|\boldsymbol{\delta}\| = \Theta(1/\sqrt{d})$ .

Using this plausible assumption about the scaling of strategy distributions, we can re-estimate the covariance:

$$|\text{Cov}(M_i, M_j)| \approx |\boldsymbol{\delta}_i^\top \boldsymbol{\Sigma}_{\text{payoff}} \boldsymbol{\delta}_j| \quad (\text{I.23})$$

$$\leq L^2 \cdot \|\boldsymbol{\delta}_i\|_2 \|\boldsymbol{\delta}_j\|_2 \cdot \|\boldsymbol{\Sigma}_{\text{payoff}}\|_2 \quad (\text{I.24})$$

$$\approx L^2 \cdot O\left(\frac{1}{\sqrt{d}}\right) \cdot O\left(\frac{1}{\sqrt{d}}\right) \cdot O(1) = O\left(\frac{L^2}{d}\right). \quad (\text{I.25})$$

$$(\text{I.26})$$

Even in the general case, combining with the typical behavior of strategy scaling, the covariance still decays at a rate of  $O(L^2/d)$ . The correlation coefficient:

$$\rho_M = O\left(\frac{L^2}{d}\right) \quad (\text{I.27})$$

(under the assumption  $\|\boldsymbol{\delta}\| = \Theta(1/\sqrt{d})$  leading to an effective  $1/\sqrt{d}$  term).

c) Case 2.3: Random Anti-symmetric Matrix: If  $\mathbf{R}$  is randomly generated (e.g.,  $R_{ij}$  i.i.d. Rademacher for  $i < j$ ), according to random matrix theory (similar to Wigner/Girko laws), typically :

$$\lambda_{\max}(\mathbf{R}\mathbf{R}^\top) = \Theta(d) \quad (\text{I.28})$$

This leads to

$$\|\boldsymbol{\Sigma}_{\text{payoff}}\|_2 = \Theta(1/\sqrt{d}) \quad (\text{I.29})$$

and the decay rate might be even faster.

Corollary C.13 (Effect on Averaged Scores ). The sample averaging process further dilutes the covariance:

$$|\text{Cov}(G_i, G_j)| \leq \frac{|\text{Cov}(M_i, M_j)|}{n} \quad (\text{I.30})$$

Considering that the samples used to compute  $G$  are independent of the latent variable  $C$  that couples  $M_i, M_j$ . More precisely,  $G_i$  is an average of  $n$  evaluations. If these evaluations are against  $n$  independently drawn opponents or involve  $n$  independent instances of randomness for  $C$ , this holds. Therefore, the maximum correlation coefficient:

$$\rho_G := \max_{i \neq j} |\text{Cov}(G_i, G_j)| = O\left(\frac{L^2}{nd}\right). \quad (\text{I.31})$$

When using Hoeffding or Bernstein-type inequalities to analyze the sum  $S = \sum_{k=1}^m X_k$  of  $m$  weakly dependent random variables  $X_1, \dots, X_m$ , one can use extended versions for weakly dependent sequences, or consider the effective sample size  $m$  to be reduced to:

$$m' \approx \frac{m}{1 + C' \cdot m \cdot \rho / \text{Var}(X)} \quad (\text{I.32})$$

where  $\rho$  is the maximum covariance ( $\rho_M$  or  $\rho_G$ ).

Theorem C.14 (Large Deviation Correction ). Since:

$$\rho_M = O(L^2/d) \quad (\text{I.33})$$

$$\rho_G = O(L^2/(nd)) \quad (\text{I.34})$$

as long as  $d$  or  $n$  is sufficiently large such that  $m\rho$  is a small quantity relative to  $m \cdot \text{Var}(X)$  (which is typically  $O(m)$ ), then  $m' \approx m$ . This implies that the tail probability bounds have the same asymptotic order as in the independent case (e.g.,  $\exp(-\Theta(m\epsilon^2))$ ). Weak correlation primarily affects the constant factor in front of the exponential term or introduces a small lower-order correction term, without changing the core exponential decay behavior.

Theorem C.15 (Summary of Weak Correlation in SCG Framework ). In the Strictly Competitive Game framework:

- The equivalent (approximate) anti-symmetric zero-sum game structure is central to the weak correlation analysis.
- For many important scenarios (satisfying structure  $(\star)$ ), it can be rigorously proven that the covariance between  $M_i, M_j$  induced by shared latent variables decays with dimension  $d$  at a rate of  $O(L^2/d)$ .
- For more general SCGs, combining with the typical scaling properties of strategy distributions in high-dimensional spaces ( $\|\delta\| = \Theta(1/d)$  effectively), the covariance still decays at a rate of  $O(L^2/d)$ .
- For averaged scores  $G_i, G_j$ , the covariance is further diluted by the sample size  $n$ , reaching  $O(L^2/(nd))$ .

This rapidly decaying weak correlation, derived rigorously or under plausible assumptions, provides a solid theoretical foundation for the "approximate independence" assumption used in the MGM convergence proofs. All large deviation analyses based on Hoeffding/Bernstein (such as ranking stability, convergence speed bounds) remain valid in terms of order.

Corollary C.16 (Validity of Large Deviation Inequalities for MGM ). The large deviation inequalities relied upon in the theoretical analysis of the MGM algorithm are reasonable and effective within the SCG framework, and their conclusions are highly credible. This indicates that Assumption B.1, B.2 and B.3 is reasonable.

#### D. Stability of Ranking for Fixed-Weight Individuals

Definition D.1 (Ranking Reversal Event for fixed-weight individuals). Event  $\mathcal{E}_1$  satisfies:

$$\mathcal{E}_1 := \{\Delta M_{ij} > 0 \text{ and } F_j > F_i \text{ when } w_i = w_j = w_0\} \quad (\text{I.35})$$

Let  $\eta := \frac{w}{1-w} = 9, \varepsilon_0 := \frac{l}{\eta}$

Lemma D.2 (Narrow Band Probability for  $\Delta M$ ). For any  $\varepsilon > 0$ , there exists:

$$P(|\Delta M| \leq \varepsilon) \leq 2c_M \varepsilon \quad (\text{I.36})$$

Lemma D.3 (Upper Bound on the Density of  $\Delta M$ ). The density of  $\Delta M$ , denoted as  $g(x) = f_{\Delta M}(x)$ , satisfies  $g(x) \leq c_M$

Proof:

$$g(x) = \int f_M(y+x)f_M(y)dy \leq c_M \int f_M(y)dy = c_M \quad (\text{I.37})$$

□

Lemma D.4 (Hoeffding's Inequality [1]). Let  $Y_r := X_{j,r} - X_{i,r} \in [-l, l]$ , be independent with  $\mathbb{E}[Y_r] = 0$  Then for any  $t > 0$ :

$$P(\Delta G \geq t) = P\left(\frac{1}{k} \sum Y_r \geq t\right) \leq \exp\left(-\frac{kt^2}{2l^2}\right) \quad (\text{I.38})$$

Corollary D.5.

$$P(\Delta G \geq \eta x) \leq \exp\left(-\frac{k\eta^2 x^2}{2l^2}\right) \forall x > 0 \quad (\text{I.39})$$

Theorem D.6 (Stability for Fixed-Weight Individuals). We need to prove that  $P(\mathcal{E}_1) \rightarrow 0$  as the number of evaluation games  $k$  for each individual increases.

Proof:

Consider the necessary condition for a ranking flip:

$$F_j \geq F_i \Leftrightarrow (1-\omega)\Delta G \geq \omega\Delta M \Leftrightarrow \Delta G \geq \eta\Delta M \quad (\text{I.40})$$

Also

$$0 \leq \Delta G \leq l \Rightarrow 0 < \Delta M \leq \varepsilon_0 \quad (\text{I.41})$$

Thus

$$\mathcal{E}_1 \subset \{0 < \Delta M \leq \varepsilon_0 \text{ and } \Delta G \geq \eta\Delta M\} \quad (\text{I.42})$$

Bounding the Probability of a Ranking Flip:

$$P(\mathcal{E}_1) = \int_0^{\varepsilon_0} P(\Delta G \geq \eta x | \Delta M = x) g(x) dx \quad (\text{I.43})$$

1) From Lemma D.3, we have :

$$g(x) \leq c_M \quad (\text{I.44})$$

2) Assumption B.3 gives independence, so the conditional probability  $P_{condition}$  satisfies:

$$P_{condition} = P(\Delta G \geq \eta x) \quad (\text{I.45})$$

Substituting from Corollary D.5:

$$P(\mathcal{E}_1) \leq c_M \int_0^{\varepsilon_0} \exp(-ax^2) dx \quad (\text{I.46})$$

where  $a := \frac{k\eta^2}{2l^2}$ .

Calculating the Gaussian-like integral:

$$\int_0^{\varepsilon_0} e^{-ax^2} dx = \frac{\sqrt{\pi}}{2\sqrt{a}} \cdot \text{erf}(\sqrt{a}\varepsilon_0) \quad (\text{I.47})$$

Since  $\text{erf}(z) \leq 1$  and  $\sqrt{a}\varepsilon_0 = \sqrt{\frac{k}{2}}$ , we have:

$$P(\mathcal{E}_1) \leq c_M \cdot \frac{\sqrt{\pi}}{2\sqrt{a}} = c_M \cdot \frac{\sqrt{\pi}}{2} \cdot \frac{l}{\eta\sqrt{k}} \quad (\text{I.48})$$

$$P(\mathcal{E}_1) \leq \frac{c_M l \sqrt{\pi}}{\sqrt{2}\eta\sqrt{k}} \quad (\text{I.49})$$

That is:

$$P(\mathcal{E}_1) = O(1/\sqrt{k}) \quad (\text{I.50})$$

Therefore, with the number of evaluation games  $k \rightarrow \infty$ , the possibility of ranking reversal event for fixed-weight individuals will decay to 0. This ensures that the overall selection direction of the MGM during fixed-weight phase is aligned with the baseline fitness, thus maintaining a stable search drive.  $\square$

Remark D.7 (Parameter Sensitivity of  $w$ ). Theorem D.6 indicates that as the number of evaluation games  $k$  for each individual increases, the probability of a ranking flip decreases at a rate of  $O(1/\sqrt{k})$ , and parameters  $\omega$  effects the upper bound of  $P(\mathcal{E}_1)$  with  $\eta = \frac{\omega}{1-\omega}$ .

Considering the relationship of  $\omega$  and  $\eta$ :

- $\omega = 0.5, \eta = 1$
- $\omega = 0.8, \eta = 4$
- $\omega = 0.9, \eta = 9$
- $\omega = 0.99, \eta = 99$

As the  $\omega$  increases, the value of  $\eta$  grows non-linearly, and the upper bound of the flip probability decreases rapidly.

Define the sensitivity  $S(\omega)$  as the relative rate of change of the upper bound of the flip probability with respect to  $\omega$ :

$$S(\omega) = \frac{\omega}{P(\mathcal{E}_1)} \cdot \frac{dP(\mathcal{E}_1)}{d\omega} \quad (\text{I.51})$$

$$S(\omega) = -\frac{\omega}{(1-\omega)^2} = -\frac{\eta}{1-\omega} \quad (\text{I.52})$$

This indicates that:

- As  $\omega \rightarrow 1$ , sensitivity  $|S(\omega)| \rightarrow \infty$ , indicating a super high sensitivity.
- When  $\omega = 0.9$ ,  $S(\omega) = -90$ , indicating a relatively high sensitivity .
- When  $\omega = 0.5$ ,  $S(\omega) = -2$ , the sensitivity is low.

Comparing the relative upper bounds of the flip probability for different values of  $\omega$  (with  $\omega = 0.5$  as the baseline):

- $w = 0.5 \rightarrow$  Relative upper bound = 1
- $w = 0.8 \rightarrow$  Relative upper bound =  $\frac{1}{4}$
- $w = 0.9 \rightarrow$  Relative upper bound =  $\frac{1}{9}$
- $w = 0.99 \rightarrow$  Relative upper bound =  $\frac{1}{99}$

We recommend that  $\omega = 0.9$  as the suitable parameter for the reasons:

- 1) Maintaining search direction: It provides sufficiently strong baseline directional guidance.
- 2) Allowing moderate exploration: It permits a 10% influence from generalization fitness, facilitating moderate exploration.

#### E. Stability of Ranking for Dynamic-Weight Individuals

Definition E.1 (Ranking Reversal Event for dynamic-weight individuals).

$$\mathcal{E}_2 := \{F_i > F_j | \Delta_M > 0, M_i > l, M_j > l, G_i < l, G_j < l\} \quad (\text{I.53})$$

Where:

$$\Delta_M = M_j - M_i \quad (\text{I.54})$$

$$\Delta_G = G_i - G_j \quad (\text{I.55})$$

Give the dynamics weight adjust function:

Definition E.2.

$$\omega_i = \alpha(\beta) = \begin{cases} \omega & \beta < 0 \\ \omega - (\omega - 0.5)(1 - e^{-v\beta}) & \beta \geq 0 \end{cases} \quad (\text{I.56})$$

Where:

$$\beta = M_i - l \quad (\text{I.57})$$

$$\sigma = G_i - l \quad (\text{I.58})$$

$$v = -\min(0, \sigma) \geq 0 \quad (\text{I.59})$$

And the fitness of individual  $i$  is:

$$F_i = \omega_i M_i + (1 - \omega_i) G_i \quad (\text{I.60})$$

Theorem E.3 (Stability of Ranking for Dynamic-Weight Individuals). Proof:

Considering the algebraic necessary condition for event  $\mathcal{E}_2$ :

$$F_i > F_j \implies (1 - \omega_i) G_i - (1 - \omega_j) G_j > \omega_j M_j - \omega_i M_i \quad (\text{I.61})$$

Let  $\omega_j = \gamma + \omega_i$ , we have:

$$\Delta_G > \frac{\omega_i \Delta_M + \gamma(M_j - G_j)}{1 - \omega_i} \quad (\text{I.62})$$

Since  $M_j - G_j \in (0, 1)$ ,  $\gamma \in (0.5 - \omega, \omega - 0.5)$

$$\frac{\omega_i \Delta_M + \gamma(M_j - G_j)}{1 - \omega_i} > \frac{\omega_i \Delta_M}{1 - \omega_i} - \frac{\omega - 0.5}{1 - \omega_i} \quad (\text{I.63})$$

That is

$$\Delta_G > \frac{\omega \Delta_M}{1 - \omega} - \frac{\omega - 0.5}{1 - \omega} \quad (\text{I.64})$$

Let  $\omega = 0.9$

$$\Delta_G > 9\Delta_M - 4 \quad (\text{I.65})$$

From Lemma D.3 and D.4, we have

$$P(\Delta_G > 9\Delta_M - 4) \leq \exp\left(-\frac{k(9\Delta_M - 4)^2}{2}\right) \quad (\text{I.66})$$

Thus

$$P(\mathcal{E}_2) \leq \int_0^{0.1} f_{\Delta_M}(x) P(\Delta_G > 9x - 4) dx \quad (\text{I.67})$$

Let  $y = 9x - 4$ , when  $x \in (0, 0.1)$ ,  $y \in (-4, -3.1)$ :

$$P(\mathcal{E}_2) \leq \int_{-4}^{-3.1} \exp\left(-\frac{k}{2}y\right) dy \quad (\text{I.68})$$

Recall the Gaussian integral:

$$\int e^{-ky^2/2} dy = \sqrt{\frac{\pi}{2k}} \operatorname{erf}\left(\sqrt{\frac{k}{2}} y\right) \quad (\text{I.69})$$

where  $\operatorname{erf}(\cdot)$  is the error function. Applying this to the bounds, we get

$$P(\mathcal{E}_2) = \frac{C_M}{9} \sqrt{\frac{\pi}{2k}} \left[ \operatorname{erf}\left(4\sqrt{\frac{k}{2}}\right) - \operatorname{erf}\left(3.1\sqrt{\frac{k}{2}}\right) \right] \quad (\text{I.70})$$

Therefore,  $\lim_{k \rightarrow \infty} P(\mathcal{E}_2) = 0$ , decaying at a rate of  $O(1/\sqrt{k})$ .  $\square$

## F. Stability of Ranking for Dynamic-Weight And Fixed-Weight Individuals

Definition F.1 (Cross-set ranking flip event).

$$\mathcal{E}_3 := \{F_D > F_S \text{ and } \Delta_M > 0\} \quad (\text{I.71})$$

Among them,  $F_D$  represents the fitness of an individual whose  $\omega$  is dynamic,  $F_S$  represents the fitness of an individual whose  $\omega$  is fixed,  $\Delta_M$  represents the difference of  $M_S$  and  $M_D$ .

$$F_D = \alpha \cdot M_D + (1 - \alpha)G_D \quad (\text{I.72})$$

$$F_s = \omega \cdot M_S + (1 - \omega)G_S \quad (\text{I.73})$$

$$\Delta_M = M_S - M_D \quad (\text{I.74})$$

$$\Delta_G = G_D - G_S \quad (\text{I.75})$$

Let the flip probability for a single pair  $(S, D)$  be denoted as:

$$P(k) := P(\mathcal{E}_3) \quad (\text{I.76})$$

Lemma F.2 (Large Deviation Bound for the Dynamic Weight). Proof:

From Lemma D.3 and Lemma D.4 and Definition E.2, large deviation bound for the dynamic weight:

$$\alpha(\beta, \sigma) = \omega - \Delta w_{max}(1 - e^{-(\sigma)^\beta}), \quad \Delta w_{max} = 0.4 \quad (\text{I.77})$$

where:

$$\sigma := (1/k) \sum_{i=1}^k u_1(p_i, p_k) - l \quad (\text{I.78})$$

It is clearly that  $\mathbb{E}(u_1(p_i, p_k) - l) \leq 0$ . Hoeffding's inequality gives :

$$P(-\sigma \geq u) \leq \exp(-ku^2/2), \quad u \geq 0 \quad (\text{I.79})$$

We introduce the variable  $\gamma$  as the minimum decrease of  $\alpha$  relative to  $\omega$ :

$$\alpha \leq \omega - \gamma \quad (\text{I.80})$$

With Eq I.77 and I.78, we have:

$$\Delta w_{max}(1 - e^{-(\sigma)\beta}) \geq \gamma \quad (\text{I.81})$$

$$e^{-(\sigma)\beta} \leq 1 - \frac{\gamma}{\Delta w_{max}} \quad (\text{I.82})$$

$$-\sigma \geq -\frac{1}{\beta} \ln(1 - \frac{\gamma}{\Delta w_{max}}) \quad (\text{I.83})$$

Here,  $\beta < 1$  and  $-\ln(1 - x) \leq -x$ :

$$-\sigma \geq \frac{\gamma}{\Delta w_{max}} \quad (\text{I.84})$$

Substituting into Eq I.79 gives:

$$P(\alpha \leq \omega - \gamma) \leq \exp\left(\frac{k\gamma^2}{2\Delta w_{max}^2}\right) \quad (\text{I.85})$$

□

Considering algebraic necessary condition for a flip:  $\Delta_M > 0$  and  $F_D > F_S$ , we have:

$$(1 - \alpha)\Delta_G > \gamma(M_S - M_D) + \alpha\Delta_M \quad (\text{I.86})$$

Since  $|M_S - G_S| \leq 1$  and  $\alpha \leq \omega$ ,

$$\Delta_G > \frac{\omega\Delta_M - \gamma(1 + \Delta_M)}{1 - \omega} \quad (\text{I.87})$$

Let  $\omega = 0.9, 1 - \omega = 0.1$ , we have:

$$\Delta_G > 10[0.9\Delta_M - \gamma(1 + \Delta_M)] \quad (\text{I.88})$$

Note: Eq I.87 and Eq I.88 are not the tightest bounds but are sufficient as necessary conditions. We divide event  $\mathcal{E}_3$  into events  $\mathcal{A}_1$  and  $\mathcal{A}_2$ , each defined as follows:

Definition F.3 (Event  $\mathcal{A}_1$ ).

$$\mathcal{A}_1 := \{\gamma \geq t\Delta_M\} \quad (\text{I.89})$$

Definition F.4 (Event  $\mathcal{A}_2$ ).

$$\mathcal{A}_2 := \{\gamma < t\Delta_M\} \quad (\text{I.90})$$

With Definition F.3 and F.4, we set  $t = \Delta w_{max}$ :

$$\mathcal{E}_3 \subset \mathcal{A}_1 \cup \mathcal{A}_2 \quad (\text{I.91})$$

Theorem F.5 (Stability for Cross Set Individuals). Proof: Step1: Upper Bound on the Probability of Event  $\mathcal{A}_1$

Since  $\gamma \geq t\Delta_M \Rightarrow \alpha \leq \omega - t\Delta_M$ :

$$P(\mathcal{A}_1) \leq \int_0^1 f_{\Delta_M}(x) Pr(\alpha \leq \omega - tx) dx \quad (\text{I.92})$$

$$\leq c_\Delta \int_0^1 \exp(-kt^2x^2/(2\Delta w_{max}^2)) dx \quad (\text{I.93})$$

Let  $a := kt^2/(2\Delta w_{max}^2)$ , with

$$\int_0^1 e^{-ax^2} dx \leq \sqrt{\pi}/(2\sqrt{a}) \quad (\text{I.94})$$

We have

$$P(\mathcal{A}_1) \leq c_M \frac{\sqrt{\pi} \Delta w_{max}}{2t\sqrt{k}} \quad (\text{I.95})$$

Step2:Upper Bound on the Probability of Event  $\mathcal{A}_2$

Since  $\gamma < t\Delta M$ , with Eq I.88:

$$\Delta_G > 10[0.9\Delta_M - \gamma(1 + \Delta_M)] > 10[0.9\Delta_M - t\Delta_M(1 + \Delta_M)] \quad (\text{I.96})$$

That is:

$$\Delta_G > 10\Delta_M(0.5 - 0.4\Delta_M) \quad (\text{I.97})$$

We noticed that:

$$10\Delta_M(0.5 - 0.4\Delta_M) - \Delta_M = 4\Delta_M(1 - \Delta_M) \quad (\text{I.98})$$

Since  $0 < \Delta_M < 1$ , we have:

$$\Delta_G > 10\Delta_M(0.5 - 0.4\Delta_M) > \Delta_M \quad (\text{I.99})$$

It is clearly that

$$\mathcal{A}_2 := \{\Delta_G > 10\Delta_M(0.5 - 0.4\Delta_M)\} \subset \mathcal{A}_3 := \{\Delta_G > \Delta_M\} \quad (\text{I.100})$$

Thus

$$P(\mathcal{A}_2) \leq P(\mathcal{A}_3) \quad (\text{I.101})$$

$$P(\mathcal{A}_2) \leq P(\mathcal{A}_3) \leq \int_0^1 f_{\Delta_M}(x) P(\Delta G > x) dx \quad (\text{I.102})$$

$$\leq c_M \int_0^1 \exp(-2kx^2) dx \leq \frac{c_M}{\sqrt{2k}} \quad (\text{I.103})$$

Step3:Aggregation

From Eq I.76,I.91,I.95,I.103, we have:

$$P(k) \leq c_M \frac{\sqrt{\pi} \Delta w_{max}}{2t\sqrt{k}} + \frac{c_M}{\sqrt{2k}} = \frac{C}{\sqrt{k}} \quad (\text{I.104})$$

Where:

$$C := c_M \left[ \frac{1}{\sqrt{2}} + \frac{\sqrt{\pi}}{2} \right] \quad (\text{I.105})$$

Therefore,  $\lim_{k \rightarrow \infty} P(k) = 0$ , decaying at a rate of  $O(1/\sqrt{k})$ . From Theorem D.6,E.3, we have:

□

Remark F.6 (Punishing Overfitting / Rewarding Generalization). • Two rare pathways lead to a flip:

- 1)  $\mathcal{A}_1$ : Significant downward adjustment of the dynamic weight: probability upper bound (Eq I.95).
  - 2)  $\mathcal{A}_2$ : Generalization score exhibits an  $O(\sqrt{k})$  level deviation: upper bound of probability (Eq I.103).
- The flip probabilities of the same order  $O(\sqrt{k})$  have previously been derived for the cases 'Stable - stable' and 'Dynamic - dynamic' (Theorem D.6 and E.3) have been derived previously; combining all three types of scenarios yields  $P(k) = O(\sqrt{k}) \rightarrow 0$
  - The  $\mathcal{A}_1$  Pathway: The 'Penalize Overfitting' Mechanism
    - 1) From Definition E.2, where  $\Delta\omega_{max} = 0.4, \omega = 0.9$ . If  $\beta > 0$ , then  $\alpha < \omega$ , and the larger  $\beta$  is, the smaller  $\alpha$  becomes. The triggering condition for  $\mathcal{A}_1$ :  $\gamma = \omega - \alpha \geq t\Delta_M$  (where  $t = 0.4$ ), implies: This indicates a large  $\beta$ , meaning excessively high base fitness  $\rightarrow$  potential overfitting.
    - 2) At this point, if generalized fitness stays at a lower level,  $\alpha$  is forcibly suppressed  $\Rightarrow$  The composite fitness  $F_i = \alpha M_i + (1 - \alpha)G_i$  becomes less dependent on  $M_i$ , and the penalty on  $G_i$  is amplified.
  - The  $\mathcal{A}_2$  Pathway: The 'Reward High Generalization' Mechanism

- 1) The triggering condition for  $\mathcal{A}_2: \gamma < t\Delta_M$  and  $\Delta_G > \Delta_M$  (where  $t = 0.4$ ), can be rewritten as:

$$G_D - G_S > M_S - M_D \geq \frac{\gamma}{t} \quad (\text{I.106})$$

This means that when  $\alpha$  is only slightly adjusted downwards, a flip occurs only if the 'generalization advantage'  $\Delta_G$  of the dynamic individual  $D$  is sufficient to cover its entire marker disadvantage  $\Delta_M$ .

- 2) In other words: If individual  $D$  relies solely on high base fitness ( $M_D \uparrow, G_D \downarrow$ ), it is difficult to satisfy Eq I.106. In contrast, if  $D$  has learned a transferable 'excellent pattern' ( $G_D \uparrow$ ), then Eq I.106 is easily to be satisfied. Therefore  $\mathcal{A}_2$  acts as a 'positive filter': it automatically promotes individuals with genuinely superior generalization to the elite ranks, providing high-quality pattern fragments for subsequent evolution; this is crucial for escaping local optima and avoiding premature convergence.

- Combined Effect and Premature Convergence Avoidance

- 1)  $\mathcal{A}_1$ : 'Hard Penalty' driven by high  $\beta$ :
  - a) Rapidly reduces the selection probability of overtly overfitted individuals.
  - b) Prevents individuals with artificially inflated training scores from occupying elite slots.
- 2)  $\mathcal{A}_1$ : 'Positive Incentive' driven by large  $\Delta_G$ :
  - a) Allows individuals with generalization capabilities significantly superior to the average to stand out.
  - b) Enhances population diversity and maintains search momentum.
- 3) These two pathways, one penalizing and one rewarding, collaboratively regulate population ranking, enabling MGM to maintain moderate exploration and selection pressure even during the marker gene stabilization phase, significantly reducing the probability of getting trapped in premature local optima.

## G. Probability of Old Marker Gene Outperforming New Marker Gene (Event $\mathcal{E}$ )

Lemma G.1 (the Relationship Between the Two Fitness Components and the Target Fitness). From Definition E.2, it is known that  $\alpha \in [0.5, \omega]$ . If  $M \leq l$  and  $G \leq l$ , we have:

$$F_i \leq \alpha \cdot l + (1 - \alpha) \cdot l = l \quad (\text{I.107})$$

This indicates that for the comprehensive fitness  $F_i$  to be strictly greater than  $l$ , at least one fitness component must be strictly greater than  $l$ . This conclusion is independent of whether the weights are constant, as long as  $\alpha \geq 0.5$ . Therefore,  $F_i > l$  for  $K$  consecutive generations is actually equivalent to at least one component ( $M_i$  or  $G_i$ ) is greater than  $l$  for  $K$  consecutive generations.

Lemma G.2 (Constraints on the Old Marker Gene). Before triggering an update, the system requires :

$$\bigwedge_{s=t}^{t+K-1} \frac{|i \in \text{Pop}_s \mid F(i, s) > l|}{N_{pop}} \geq 75\% \quad (\text{I.108})$$

where  $t$  is the generation number,  $\text{Pop}_t$  is the set of individuals in generation  $t$ . Representing Eq I.108 using an indicator variable:

$$X_{i,t} = \mathbf{1}\{\max(M(i, t), G(i, t)) > l\} \quad (\text{I.109})$$

If for the old marker gene  $p_{old} = P(X = 1)$  (the probability of success in a single independent trial), then the number of successes in each generation  $S \sim \text{Binom}(N_{pop}, p_{old})$ . For  $S \geq 0.75N_{pop}$  to occur for  $K$  consecutive times, according to the Chernoff inequality [2] :

$$P(S \geq 0.75N_{pop}) \leq \exp[-N_{pop}D(0.75p_{old})] \quad (\text{I.110})$$

Where  $D(\cdot)$  is the KL divergence. Multiplying I.110  $K$  times yields:

$$P\left(\bigwedge_{s=t}^{t+K-1} \frac{|i \in \text{Pop}_s \mid F(i, s) > l|}{N_{pop}} \geq 75\% \mid p_{old}\right) \leq \exp[-KN_{pop}D(0.75p_{old})] \quad (\text{I.111})$$

If the right-hand side is controlled to be a very small value to  $\epsilon$  (e.g.,  $10^{-4} \sim 10^{-6}$ ), and use Taylor to expand the approximation, then we have:

$$p_{\text{old}} \geq 0.75 + \delta_{\text{old}}, \quad \delta_{\text{old}} \gtrsim \frac{\sqrt{3}}{2} \sqrt{\frac{\ln(1/\epsilon)}{KN_{\text{pop}}}} \gtrsim \Omega \left( \sqrt{\frac{\ln(1/\epsilon)}{KN_{\text{pop}}}} \right) \quad (\text{I.112})$$

Further analyzing according to Lemma G.1, for  $X_i = 1$ , it is at least required that:

$$P(G_{\text{old}} > l) \geq p_{\text{old}} - P(M_{\text{old}} > l) \quad (\text{I.113})$$

In the most conservative case, where  $M_{\text{old}} = 1$ , we still have:

$$P(G_{\text{old}} > l) \geq 0.75 + \delta_{\text{old}} - 1 = -0.25 + \delta_{\text{old}} \quad (\text{I.114})$$

As long as  $\delta_{\text{old}} \geq 0.26$  (when  $N_{\text{pop}} = 50, K = 3, \delta_{\text{old}} \approx 0.3$ ), Eq I.114 implies that  $G_{\text{old}}$  must also frequently be higher than  $l$ . Therefore, the true generalization mean of the old marker gene,  $\mu_{\text{old}}$  must be at least a safety distance  $\Delta_{\text{old}}$ .

Lemma G.3 (Constraints on the New Marker Gene). The new marker gene needs to satisfy in its self-play:

$$F_{\text{new}}(t) > l, \quad t = 1, \dots, K \quad (\text{I.115})$$

Since only its own performance is considered, the statistical strength of Eq I.115 is higher: the probability of  $K$  consecutive successes  $\leq (1 - p_{\text{new\_fail}})^K$ . Similarly, by setting  $\epsilon$  to be very small, we get:

$$P(G_{\text{new}} > l) \geq 1 - \epsilon^{1/K} = 1 - \epsilon' \quad (\text{I.116})$$

This pushes  $\mu_{\text{new}}$  to a value  $\Delta_{\text{new}}$  above  $l$ .

Combining Eq I.112, I.113, I.114, I.116:

$$\mu_{\text{new}} \geq l + \Delta_{\text{new}}, \quad \mu_{\text{old}} \leq l - \Delta_{\text{old}} \Rightarrow \delta^* := \mu_{\text{new}} - \mu_{\text{old}} \geq \Delta_{\text{old}} + \Delta_{\text{new}} \quad (\text{I.117})$$

Definition G.4 (Event that Old Marker Gene Outperforming New Marker Gene). Event  $\mathcal{E}$  can be defined as:

$$\mathcal{E} := \{G_{\text{old}} > G_{\text{new}} \mid \bigwedge_{s=t}^{t+K-1} \frac{|i \in \text{Pop}_s \mid F(i, s) > l|}{N_{\text{pop}}} \geq 75\%, \quad \bigwedge_{s=t}^{t+K-1} F_{\text{new}}(s) > l\} \quad (\text{I.118})$$

Theorem G.5 (The probability of  $\mathcal{E}$  converges to 0 bi-exponentially.). Proof: Each evaluation involves measurement noise  $\epsilon \sim \mathcal{N}(0, \tau^2)$ , where  $\tau$  is typically  $\leq 0.015$ . In the generation where the update is triggered:

$$G_{\text{old}} = \mu_{\text{old}} + \epsilon_1, \quad G_{\text{new}} = \mu_{\text{new}} + \epsilon_2, \quad \epsilon_1, \epsilon_2 \sim \text{i.i.d.} \mathcal{N}(0, \tau^2) \quad (\text{I.119})$$

Event  $\mathcal{E}$  occurs if and only if:

$$G_{\text{old}} > G_{\text{new}} \Leftrightarrow \epsilon_1 - \epsilon_2 > \delta^* \quad (\text{I.120})$$

Since  $\epsilon \sim \mathcal{N}(0, \tau^2)$ , therefore:

$$P(\mathcal{E}) = \Phi \left( -\frac{\delta^*}{\sqrt{2}\tau} \right) \quad (\text{I.121})$$

This means that when measurement noise is at common levels, the upper bound on the probability of event rapidly drops to  $10^{-3} \sim 10^{-5}$ , and decreases exponentially with  $N_{\text{pop}}$  and  $K$ ; in the limit  $\tau \rightarrow 0, P(\mathcal{E}) \rightarrow 0$ .  $\square$

## H. Local Dissipation and Stochastic Stability of MGM

Lemma H.1 (Monotonically Non-increasing of Dynamic Weighting Function). Let parameters  $\omega \in (0, 1), v > 0$ , from Definition E.2:

$$\alpha(\beta) = \begin{cases} \omega, & \beta \leq 0, \\ 0.5 + (\omega - 0.5)e^{-v\beta}, & \beta > 0. \end{cases} \quad (\text{I.122})$$

If it further satisfies:

$$\omega \geq 0.5 \quad (\text{I.123})$$

then we have  $\alpha$  is piecewise  $C^1$  with at most one kink at  $\beta = 0$ ; it is constant on  $\beta \leq 0$  and non-increasing on each connected subset of  $\{\beta > 0\}$

Proof: Direct differentiation for  $\beta > 0$  yields:

$$\alpha'(\beta) = \frac{d}{d\beta} \{0.5 + (\omega - 0.5)e^{-v\beta}\} = (\omega - 0.5)v e^{-v\beta} \quad (\text{I.124})$$

Combining with condition (I.123), we know that :

$$\alpha'(\beta) \leq 0, \quad \forall \beta > 0 \quad (\text{I.125})$$

and when  $\beta > 0, e^{-v\beta} > 0$ ; if  $\omega > 0.5$ , then  $\alpha'(\beta) < 0$ , hence monotonicity holds.

Next, we verify differentiability: the left limit

$$\lim_{\beta \rightarrow 0^-} \alpha(\beta) = \omega \quad (\text{I.126})$$

the right limit

$$\lim_{\beta \rightarrow 0^+} \alpha(\beta) = 0.5 + (\omega - 0.5) = \omega \quad (\text{I.127})$$

hence continuous.

The left derivative is  $\alpha'(0^-) = 0$ , the right derivative is  $\alpha'(0^+) = (\omega - 0.5)v$ ; when  $\omega = 0.5$ , both are equal to 0. If  $\omega > 0.5$ , a  $C^1$  extension can be constructed near  $\beta = 0$  using a standard smooth transition. Therefore,  $\alpha \in C^1(\mathbb{R})$ . The limit property :

$$\alpha(\beta) = 0.5 + (\omega - 0.5)e^{-v\beta} \xrightarrow{\beta \rightarrow \infty} 0.5 \quad (\text{I.128})$$

clearly holds. □

Lemma H.2. Let  $U := (M_i(x^*) - G_i(x^*))_{i=1}^d \in \mathbb{R}^d$ , and let  $\Sigma = \text{Cov}[U]$ . Under conditions B.5–B.7 and the antisymmetric payoff matrix assumption, there exist constants  $C, c > 0$  independent of  $d$  such that for all  $k$ ,

$$P\left\{\|\Sigma\|_2 \leq \frac{C}{d-1}\right\} \geq 1 - 2\exp(-ck). \quad (\text{I.129})$$

Proof: Step 1: Spectral Bound on True Covariance The antisymmetric game satisfies

$$\sum_{i=1}^d U_i = 0 \quad (\text{I.130})$$

making  $\mathbf{1}_d$  a null eigenvector of  $\Sigma$ . Let  $Q = I - \frac{1}{d}\mathbf{1}\mathbf{1}^\top$  be the orthogonal projection. We observe

$$\Sigma = \sigma^2 Q \quad (\text{I.131})$$

where  $\sigma^2 = \text{Var}[U_1] = \text{Var}[U_i]$  holds for all  $i$ . Since the non-zero eigenvalues of  $Q$  are all 1, we have

$$\lambda_{\max}(\Sigma) = \sigma^2 \quad (\text{I.132})$$

As  $U_i$  represents the difference of means of  $m$  bounded  $([-2, 2])$  random variables, we get  $\sigma^2 \leq \frac{8}{k}$ . Using  $m = k \geq c_0(d-1)$  from B.6 (note that  $\sqrt{k} \gtrsim d$  always holds in experiments), we obtain

$$\lambda_{\max}(\Sigma) \leq \frac{8}{c_0(d-1)} = \frac{C}{d-1}.$$

Step 2: Controlling Empirical Covariance Deviation Let  $\hat{\Sigma} = \frac{1}{m} \sum_{t=1}^m U_t U_t^\top$  be the sample covariance. By the Matrix–Bernstein inequality :

$$P\left\{\|\hat{\Sigma} - \Sigma\|_2 \geq \frac{C}{2(d-1)}\right\} \leq 2d \exp\left(-\frac{kC^2}{16(d-1)^2}\right) \leq 2\exp(-c\sqrt{k}), \quad (\text{I.133})$$

where absorbs polynomial factors of  $d$  into  $c$ . Thus,  $\|\hat{\Sigma}\|_2 \leq \frac{C}{d-1}$  holds with the same probability.  $\square$

Proposition H.3 (Old–New Marker Gap). Under Assumptions B.5–B.7 and Theorem G.5 Then for some universal constants  $C_0, c_0 > 0$ ,

$$P\{\mathcal{E}\} \leq C_0 \exp(-c_0 N_{\text{pop}} K). \quad (\text{I.134})$$

Theorem H.4 (Local Dissipation and Stochastic Stability). Let  $x^* \in \Delta^{n-1}$ , be a strictly mixed Nash equilibrium satisfying assumption B.4, B.5B.6, B.7. Let the ODE system induced by MGM in the noiseless limit ( $\mu \rightarrow 0$ ) be:

$$\dot{x}_i = x_i[F_i(x) - (x)] \quad (\text{I.135})$$

where  $\phi(x) = \sum_j x_j F_j(x)$

$$F_i(x) = \alpha(\beta(x))M_i(x) + (1 - \alpha(\beta(x)))G_i(x) \quad (\text{I.136})$$

$$\beta(x) = \sum_k x_k M_k(x) - l \quad (\text{I.137})$$

Then for any fixed, sufficiently large  $N_{\text{pop}}$  (which is positively correlated with  $k$ ) (such that Lemma H.2, H.3 holds with high probability), we have:

- 1) The ODE is locally dissipative at  $x^*$ : The divergence of the vector field at the equilibrium point  $x^*$ ,  $\text{div} F(x^*) < 0$ , indicates that the dynamical system is exponentially volume-contracting near this point, and  $x^*$  is a local attractor of this deterministic dynamical system.
- 2) Stochastic stability: Considering the stochastic process with small noise ( $\mu > 0$ ) (approximable by the diffusion process  $dX = F(X)dt + \sqrt{\mu}\sigma(X)dW$ ), according to Freidlin–Wentzell large deviation theory, the mean time  $E[T_{\text{exit}}]$  required to escape from the basin of attraction  $B$  of  $x^*$  satisfies  $E[T_{\text{exit}}] \asymp \exp(V^*/\mu)$ , where  $V^* > 0$  is the minimum quasi-potential or potential barrier height that must be overcome to escape.

Proof: Step 1: Local Dissipativity of the ODE at  $x^*$  We compute the divergence of the vector field  $F$  at the equilibrium point  $x^*$ , i.e., the trace of its Jacobian matrix  $\mathbf{J}, \text{tr}(\mathbf{J})$ . According to Lemma H.2, for sufficiently large  $N_{\text{pop}}$ , the condition  $\Delta_i = M_i(x^*) - G_i(x^*) > 0$  holds almost surely for all  $i \in \text{supp}(x^*)$ .

Lemma H.5 (Jacobian Trace Formula). At the equilibrium point  $x^*$ , the divergence of the replicator dynamics vector field  $\dot{x}_i = x_i[F_i(x) - (x)]$  is :

$$\text{div} F(x^*) = \sum_{i,j} x_i^*(\delta_{ij} - x_j^*) \cdot \frac{\partial F_j}{\partial x_i} \Big|_{x^*} \quad (\text{I.138})$$

Proof: At the equilibrium point  $x^*$ ,  $F_i(x^*) = \phi(x^*)$ . Computing the divergence:

$$\text{div} F(x) = \sum_i \frac{\dot{x}_i}{x_i} = \sum_i \frac{1}{x_i} [x_i(F_i - \phi)] \quad (\text{I.139})$$

$$= \sum_i \left[ (F_i(x) - \phi(x)) + x_i \left( \frac{\partial F_i}{\partial x_i} - \frac{\partial \phi}{\partial x_i} \right) \right] \quad (\text{I.140})$$

At  $x^*$ , the first term is zero. Continuing with the calculations:

$$\operatorname{div} F(x^*) = \sum_i x_i^* \left[ \frac{\partial F_i}{\partial x_i} \Big|_{x^*} - \sum_j \frac{\partial (x_j F_j)}{\partial x_i} \Big|_{x^*} \right] \quad (\text{I.141})$$

$$= \sum_i x_i^* \left[ \frac{\partial F_i}{\partial x_i} \Big|_{x^*} - \sum_j \left( \delta_{ij} F_j(x^*) + x_j^* \frac{\partial F_j}{\partial x_i} \Big|_{x^*} \right) \right] \quad (\text{I.142})$$

$$= \sum_i x_i^* \frac{\partial F_i}{\partial x_i} \Big|_{x^*} - \sum_i x_i^* F_i(x^*) - \sum_i \sum_j x_i^* x_j^* \frac{\partial F_j}{\partial x_i} \Big|_{x^*} \quad (\text{I.143})$$

$$= \sum_i x_i^* \frac{\partial F_i}{\partial x_i} \Big|_{x^*} - \phi(x^*) - \sum_j x_j^* \sum_i x_i^* \frac{\partial F_j}{\partial x_i} \Big|_{x^*} \quad (\text{I.144})$$

$$= \sum_{i,j} x_i^* (\delta_{ij} - x_j^*) \cdot \frac{\partial F_j}{\partial x_i} \Big|_{x^*} \quad (\text{I.145})$$

□

Lemma H.6 (Partial Derivative Calculation). For  $F_j = \alpha(\beta)M_j + (1-\alpha(\beta))G_j$ , where  $\beta(x) = \sum_k x_k M_k(x) - l$ , we have:

$$\frac{\partial F_j}{\partial x_i} \Big|_{x^*} = \alpha'(\beta^*) \cdot \frac{\partial \beta}{\partial x_i} \Big|_{x^*} \cdot [M_j(x^*) - G_j(x^*)] + \alpha^* \frac{\partial M_j}{\partial x_i} \Big|_{x^*} + (1 - \alpha^*) \frac{\partial G_j}{\partial x_i} \Big|_{x^*} \quad (\text{I.146})$$

Lemma H.7. At the equilibrium point, the divergence of the vector field can be decomposed as:

$$\operatorname{div} F(x^*) = \alpha'(\beta^*) \cdot \sum_{i,j} x_i^* (\delta_{ij} - x_j^*) \cdot M_i(x^*) \cdot [M_j(x^*) - G_j(x^*)] + C \quad (\text{I.147})$$

where  $C$  is the contribution from other terms and is zero under standard replicator dynamics.

Proof: Substitute the partial derivatives from Lemma H.6 into the divergence formula from Lemma H.5. The key is that standard replicator dynamics (if  $\alpha$  is constant) have a zero divergence property. Therefore, all terms not explicitly containing  $\alpha'(\beta^*)$  (i.e. those related to  $\alpha^* \partial M_j / \partial x_i$  and  $(1 - \alpha^*) \partial G_j / \partial x_i$ ), will sum to zero after the operation  $\sum_{i,j} x_i^* (\delta_{ij} - x_j^*) \cdot [\dots]$ . Thus,  $C = 0$ . We do this to sort out the sources of non-zero dispersion. □

Lemma H.8 (Vectorized Representation). The divergence can be expressed as a quadratic form:

$$\operatorname{div} F(x^*) = \alpha'(\beta^*) \cdot u^\top \cdot \mathbf{D} \cdot r \quad (\text{I.148})$$

where  $\mathbf{D} = \operatorname{diag}(x^*) - x^*(x^*)^\top$ ,  $u = M(x^*) \in \mathbb{R}^n$ ,  $r = M(x^*) - G(x^*) \in \mathbb{R}^n$

Lemma H.9 (Negative Divergence). From Lemma H.1, H.2, Proposition H.3 and Assumption B.4, we have:

- $\alpha'(\beta^*) < 0$
- $u_i = M_i(x^*) > 0$
- $r_i = M_i(x^*) - G_i(x^*) > 0$
- $\mathbf{D}$  is positive definite on the tangent space.

Since all components of vectors  $u$  and  $r$  are positive, their projections onto the tangent space are typically non-zero. Therefore, the quadratic form  $u^\top \mathbf{D} r > 0$ . Combining these:

$$\operatorname{div} F(x^*) = \alpha'(\beta^*) \cdot u^\top \mathbf{D} r < 0 \quad (\text{I.149})$$

Lemma H.10 (Negative Definiteness of the Symmetric Part of the Jacobian). From the MGM dynamical equations :

$$\dot{x}_i = x_i [F_i(x) - (x)] \quad (\text{I.150})$$

at the equilibrium point  $F_i(x^*) = \phi(x^*)$ , the Jacobian matrix elements are:

$$\mathbf{J}_{ij} := \frac{\partial x'_i}{\partial x_i} \Big|_{x^*} \quad (\text{I.151})$$

$$= \delta_{ij} \cdot 0 + x_i^* [\partial_j F_i - \partial_j \phi] \quad (\text{I.152})$$

$$= x_i^* \left[ \partial_j F_i - \sum_k x_k^* \partial_j F_k \right] \quad (\text{I.153})$$

expressed in matrix form:

$$\mathbf{J} = \mathbf{X}^* \cdot \mathbf{P} \cdot \mathbf{DF} \quad (\text{I.154})$$

where  $\mathbf{X}^* = \text{diag}(x^*)$ ,  $\mathbf{DF} = ((\partial_j F_i)|_{x^*})$ ,  $\mathbf{P} = \mathbf{I} - \mathbf{1} \cdot (x^*)^\top$ . From previous calculations,  $\mathbf{DF}$  at the equilibrium point can be decomposed as:

$$\mathbf{DF} = \alpha'^* \cdot u \cdot r^\top + (\alpha^* \mathbf{DM} + (1 - \alpha^*) \mathbf{DG}) \quad (\text{I.155})$$

Due to the Hamiltonian nature of the replicator dynamics part, we have :

$$\mathbf{P}(\alpha^* \mathbf{DM} + (1 - \alpha^*) \mathbf{DG}) = 0 \quad (\text{I.156})$$

thus only the following remains in  $\mathbf{P} \cdot \mathbf{DF}$ :

$$\mathbf{P} \cdot \mathbf{DF} = \alpha'^* \cdot \mathbf{P} \cdot (u \cdot r^\top) \quad (\text{I.157})$$

The Jacobian matrix can be expressed as:

$$\mathbf{J} = \mathbf{X}^* \cdot [\alpha'^* \mathbf{P} \cdot u \cdot r^\top] \quad (\text{I.158})$$

Therefore, the symmetric part  $\mathbf{S} = \mathbf{J} + \mathbf{J}^\top$ :

$$\mathbf{S} = \alpha'^* \cdot [\mathbf{X}^* \mathbf{P} u \cdot r^\top + (\mathbf{X}^* \mathbf{P} u \cdot r^\top)^\top] \quad (\text{I.159})$$

$$= 2\alpha'^* \cdot \text{sym}\{\mathbf{X}^* \cdot \mathbf{P} \text{diag}(u) \cdot \text{diag}(r)\} \quad (\text{I.160})$$

For any  $\tilde{r} \in \mathbb{R}^n$  such that  $\sum_i \tilde{r}_i = 0$  ( $\tilde{r}$  belongs to the tangent space  $T_{\Delta^{n-1}}$ ), we have:

$$\mathbf{J} + \mathbf{J}^\top = 2\alpha'^* \mathbf{X}^* \text{diag}(M_i(x^*)) \mathbf{P} \quad (\text{I.161})$$

Because  $\mathbf{P}\tilde{r} = \tilde{r}$ ,

$$\tilde{r}^\top (\mathbf{J} + \mathbf{J}^\top) \tilde{r} = 2\alpha'^* \tilde{r}^\top \mathbf{X}^* \mathbf{P} \mathbf{D} \tilde{r} \quad (\text{I.162})$$

Let  $\mathbf{M}_{\min} := \min_i M_i(x^*) > 0$ , we have:

$$\tilde{r}^\top \mathbf{X}^* \mathbf{P} \mathbf{D} \tilde{r} = \sum_i x_i^* M_i(x^*) \tilde{r}_i^2 \geq \mathbf{M}_{\min} \sum_i x_i^* \tilde{r}_i^2 \quad (\text{I.163})$$

Let  $\mathbf{DX} := \text{diag}(x^*) - x^*(x^*)^\top$ , because  $\tilde{r} \perp \mathbf{1}$ , we have:

$$\sum_i x_i^* \tilde{r}_i^2 = \tilde{r}^\top \mathbf{DX} \tilde{r} \quad (\text{I.164})$$

Let  $\lambda_2(\Delta) > 0$  is the smallest non-zero eigenvalue of matrix  $\Delta$ . Rayleigh's quotient gives

$$\tilde{r}^\top \mathbf{DX} \tilde{r} \geq \lambda_2(\mathbf{DX}) \|\tilde{r}\|^2. \quad (\text{I.165})$$

Since  $\alpha'^* < 0$ :

$$\tilde{r}^\top (\mathbf{J} + \mathbf{J}^\top) \tilde{r} \leq 2\alpha'^* \mathbf{M}_{\min} \tilde{r}^\top \mathbf{DX} \tilde{r} \quad (\text{I.166})$$

$$\leq 2\alpha'^* \mathbf{M}_{\min} \lambda_2(\mathbf{DX}) \|\tilde{r}\|^2 \quad (\text{I.167})$$

Thus the above expression is strictly negative.

Corollary H.11 (Local Attractiveness).  $\text{div } F(x^*) < 0$  proves that near  $x^*$ , the deterministic dynamical system is volume-contracting, and  $x^*$  is a local attractor and is locally exponentially stable.

## Step 2: Noisy Approximation and the Freidlin–Wentzell Large Deviation Framework

Lemma H.12 (SDE Approximation ). When considering a finite population  $N_{pop}$  and an effective noise intensity  $\mu = O(1/N_{pop})$ , the discrete-time evolution of MGM can be approximated by a Stochastic Differential Equation :

$$dX_t = F(X_t)dt + \sqrt{\mu}\sigma(X_t)dW_t \quad (\text{I.168})$$

where  $F(X)$  is the deterministic drift term analyzed in Step 1,  $\sigma(X)$  is the state-dependent diffusion matrix (satisfying the non-degeneracy condition Proposition H.3), and  $W_t$  is a Wiener process.

Lemma H.13. According to Freidlin–Wentzell theory, for an SDE system with a local attractor  $x^*$  (basin of attraction denoted by  $B$ ), starting near  $x^*$ , the mean time to first exit the basin  $B$ ,  $E_x[T_{exit}(B)]$  satisfies in the small noise limit:

$$\lim_{\mu \rightarrow 0} \mu \log E_x[T_{exit}(B)] = V^* \quad (\text{I.169})$$

where  $V^* = \min_{y \in \partial B} V(x^*, y) > 0$  is the minimum quasi-potential that must be overcome to reach the boundary  $\partial B$  from  $x^*$ . This implies that the mean escape time grows exponentially as the noise intensity  $\mu$ :  $E_x[T_{exit}(B)] \asymp \exp(V^*/\mu)$ .

Proof: According to the large deviation theory of Freidlin–Wentzell (F-W theory), for similar SDE systems, the escape time from an attractor satisfies the aforementioned asymptotic relationship. Since  $x^*$  has negative divergence (Corollary H.11), its local attractiveness is guaranteed, thus forming a non-empty basin of attraction  $B$ . According to F-W theory,  $V^* > 0$ , which leads to an exponentially increasing escape time.  $\square$

$\square$

## I. Global Attractiveness of the Nash Equilibrium Neighborhood

Lemma I.1 (Payoff Advantage of NE Strategies Outside  $\mathcal{N}_\epsilon$ ). For the strict NE( $S_1^*, S_2^*$ ), in the two-population game and its neighborhood  $\mathcal{N}_\epsilon$  (radius  $\epsilon$ ), there exists a constant  $c$  such that whenever the strategy distribution of at least one population lies outside  $\mathcal{N}_\epsilon$ , the NE pure strategy of that population enjoys a payoff advantage of at least  $c$  over the average fitness.

Proof: Because the NE is strict, there exist  $\varrho_1, \varrho_2$ , such that :

$$\forall S_1 \neq S_1^* \quad f_1(S_1, S_2^*) \leq f_1(S_1^*, S_2^*) - \Delta_1 \quad (\text{I.170})$$

$$\forall S_2 \neq S_2^* \quad f_2(S_1^*, S_2) \leq f_2(S_1^*, S_2^*) - \Delta_2 \quad (\text{I.171})$$

$$(\text{I.172})$$

By continuity of the payoff functions, there exist  $\epsilon > 0$  and  $\rho_1, \rho_2 > 0$ , such that when the mixed strategy  $\theta_2$  of the second population is at least  $\epsilon$  away from  $\mathcal{N}_{\epsilon_2}^*$  still holds.

$$f_1(S_1^*, \theta_2) - \max_{S_1} f_1(S_1, \theta_2) \geq \rho_1 \quad (\text{I.173})$$

Similarly, when  $\theta_1$  is at least  $\epsilon$  away from  $\sigma_2^*$  holds:

$$f_2(\theta_1, S_2^*) - \max_{S_2} f_2(\theta_1, S_2) \geq \rho_2 \quad (\text{I.174})$$

Considering the dynamic weight  $\alpha(x)$  of MGM (with  $\alpha_{min} \leq \alpha(x) \leq 1$ ), we obtain the following lower bounds on the fitness difference:

$$F_1(S_1^*, \theta_2) - \phi_1(\theta_1, \theta_2) \geq \alpha_{min} \rho_1 =: c_1 > 0, \text{ if } 22 \quad (\text{I.175})$$

$$F_2(S_2^*, \theta_1) - \phi_2(\theta_1, \theta_2) \geq \alpha_{min} \rho_2 =: c_2 > 0, \text{ if } 11 \quad (\text{I.176})$$

Let  $c := \min\{c_1, c_2\}$ , then whenever one side leaves  $\mathcal{N}_\epsilon$ , the corresponding NE pure strategy exceeds the average fitness by at least  $c$ .  $\square$

Lemma I.2 (The Time Upper Bound to Enter  $\mathcal{N}_\epsilon$ ). Under deterministic replicator dynamics, if the initial frequency of the NE pure strategy is  $\psi_0 > 0$ , the time to enter  $\mathcal{N}_\epsilon$  is bounded above by  $T_{det} := \frac{1}{c} \ln(\frac{1}{\psi_0} + 1)$ .

Proof:

Let  $\psi_*(t)$  denote the current frequency of  $S_1^*$  in the first population. According to the replicator equation

$$\dot{\psi}_* = \psi_*[F_1(S_1^*) - 1]c\psi_* \quad (\text{I.177})$$

This inequality always holds in  $\mathcal{N}_\epsilon^c$  (where  $c > 0$ ), hence

$$\frac{d}{dt} \ln(\psi_*) \geq c \Rightarrow \ln(\psi_*(t)) \geq \ln(\psi_0) + ct \quad (\text{I.178})$$

To bring the strategy distribution  $(\theta_1, \theta_2)$  into  $\mathcal{N}_\epsilon$ , it suffices that  $x_* \geq \iota$  (where  $\iota$  is a threshold for determining whether the population strategy frequency is in the NE neighborhood or not thus it is determined by  $\epsilon$ ). Setting  $\psi_0 = x_*(0)$ , reaching  $\iota$  takes at most the time:

$$t \leq T_{det} := \frac{1}{c} \ln \left( \frac{\iota}{\psi_0} \right) \leq \frac{1}{c} \ln \left[ \frac{1}{\psi_0} \right] \quad (\text{I.179})$$

The same reasoning applies to the second population; if both populations are outside  $\mathcal{N}_\epsilon$ , the two NE pure strategies grow simultaneously at rate  $\geq c$ , and the entry time into  $\mathcal{N}_\epsilon$  is still governed by the above formula.  $\square$

Lemma I.3 (Exponential Tail of the First Hitting Time). For the MGM-SDE with  $\sqrt{\epsilon}$  perturbation, the first hitting time from  $\mathcal{N}_\epsilon^c$  to  $\mathcal{N}_\epsilon$  has an exponential tail.

Proof: Consider the small-noise MGM stochastic differential equation:

$$dX = b(X)dt + \sqrt{\epsilon}\sigma(X)dW_t \quad (\text{I.180})$$

Define the set  $A_{in} := \{X \in \mathcal{N}_\epsilon^c | x_* \geq \epsilon_0\}$ . Within  $A_{in}$ , the vector field  $b(X)$  drifts against  $\ln x_*$  by at least  $c_{drift}$ , the diffusion term  $\sigma(X)$  satisfies the non-degeneracy condition (Proposition H.3, Theorem F.5). but each of its columns has bounded norm  $n_M$  on the tangent space  $T_{\Delta^{n-1}}$ . Applying the Freidlin–Wentzell large-deviation theory [3] yields: for any  $\delta \in (0, 0.5)$ , there exist constants  $q, Q > 0$  such that

$$P_x\{X_s \text{ stays in } A_{in} \forall s \in [0, (\frac{1}{c_{drift}} + \delta) \ln(\frac{1}{\epsilon_0} + 1)]\} \leq Qe^{-q/\epsilon} \quad (\text{I.181})$$

This shows that exponential growth cannot be offset by  $O(\sqrt{\epsilon})$  Gaussian perturbations for a long duration.  $\square$

Theorem I.4 (Global Attractiveness and Stochastic Stability). Summarizing the known results:

- Inside  $\mathcal{N}_\epsilon$ :  $\text{div } F(x^*) < 0$ , and the SDE escape time is  $\geq e^{V(\mathcal{N}_\epsilon)/\epsilon}$
- For the local optimum basin  $U$ , the escape time is at most polynomial.
- The entry time  $\mathcal{N}_\epsilon^c \rightarrow \mathcal{N}_\epsilon$  is  $\leq O(\log \frac{1}{\epsilon_0})$  with an  $e^{-q/\epsilon}$  tail.

Hence the unique stochastically stable set equals  $\mathcal{N}_\epsilon$  (or  $\mathcal{N}_\epsilon$  together with its arbitrarily small enlargement under noise).

Proposition I.5 (Consistency with MGM Mechanisms). The adaptive penalty mechanism of MGM does not affect the global attractiveness of  $\mathcal{N}_\epsilon$ . The following mechanisms guarantee this property:

- The old marker gene has higher generalization fitness  $\Rightarrow$  in population 2 it is hard to find strategies that both defeat  $S_1^*$  and keep an advantage over other genes.
- When a truly new high-generalization strategy emerges, after marker replacement  $\alpha(t)$  again amplifies the pressure on the opponent to 'find a nemesis', thus it can only push the system toward a new, higher-fitness local NE (if any) without causing premature stagnation.

## J. Conclusion

This proof has provided a comprehensive theoretical analysis underpinning the Marker Gene Method (MGM). We began by establishing the plausibility of the approximate independence assumption in Weak Correlation Analysis for Strictly Competitive Games, demonstrating that its validity strengthens with increasing population size ( $N_{pop}$ ) and strategy dimensionality ( $d$ ), thereby providing a robust foundation for subsequent proofs.

Next, leveraging Hoeffding’s inequality, we analyzed the population dynamics when the marker gene is fixed. We proved that under this condition, the population’s evolution can be viewed as a single-population evolution with positive perturbations, and the probability of ranking reversal events converges to zero at a rate of  $O(1/\sqrt{k})$ , where  $k$  is the number of game evaluations (positively correlated with  $N_{pop}$ ). This analysis revealed that ranking reversals are primarily driven by two pathways: (1) individuals exhibiting clear signs of overfitting (excessively high baseline fitness and low generalization fitness), or (2) individuals possessing exceptionally high generalization fitness. This insight provides the first pillar supporting the non-degeneracy condition crucial for MGM’s stability.

We then investigated the instantaneous dynamics during marker gene replacement. It was shown that the probability of an event where the old marker gene possesses superior generalization fitness compared to the new one converges to zero bi-exponentially with increases in  $N_{pop}$  and  $K$  (where  $K$  represents BufferCount and KeepCount). This finding constitutes the second pillar supporting the non-degeneracy condition.

Subsequently, employing dynamical systems theory, we proved that within a compact neighborhood of a Nash Equilibrium (NE)  $x^*$ , the divergence of the MGM flow is negative ( $\text{div } F(x^*) < 0$ ). This establishes  $x^*$  as a local attractor and demonstrates its local exponential stability. Building on this local volume contraction, we utilized Freidlin–Wentzell theory to show that, under small noise conditions, the time for the system to escape the basin of attraction of  $x^*$  is exponential.

Finally, with the non-degeneracy condition, we extended our analysis to global evolutionary dynamics. We rigorously demonstrated a crucial separation of time scales: the time to enter a compact NE neighborhood is significantly shorter than the time to leave a non-NE neighborhood, which, in turn, is significantly shorter than the time to escape the NE neighborhood itself.

## II. Details of Memory Pool (MP) Mechanism

Considering that as the number of evolutionary generations increases, the influence of the marker gene gradually diminishes, there arises a risk of re-learning previous marker genes or encountering individuals whose capabilities resemble those earlier markers. For example, the marker gene  $B_1$  in population  $B$  may successively induce markers ( $A_2, B_3, A_4, A_5 \dots B_n$ ) ;as the marker-gene updates accumulate, the dilemma introduced by  $B_1$  into population  $A$  can recur, leading to redundant learning cycles. Beyond memory decay from evolution, intransitivity can also trap the process in loops of strategy relearning. To address this cyclic issue, we draw on the concept of human experience replay and propose the Memory Pool Mechanism.

The Memory Pool Mechanism consists of two components: a memory pool and a cemetery. Each population is assigned its own memory pool and cemetery. The memory pool stores each replaced marker gene together with the most robust opponent in the population at the time of replacement; these two stored individuals form an entangled pair. An entangled object refers to the strongest adversary of a member selected into the memory pool. Upon a marker-gene update, the individual with the highest Keep Count in the population is chosen as the entangled object for that marker gene. If multiple individuals share the maximum Keep Count, the one with the highest composite fitness is selected. Before each generation begins, the individuals in the memory pool first sequentially compete against members of the opposing population, and their average fitness is computed for partitioning. Those whose fitness exceeds the target threshold are assigned to the ‘useful region’ and have their Useful Memory count incremented; those below the threshold are assigned to the “non-useful region.” Individuals in the useful region are regarded as effective memories for the current

generation and, together with their entangled objects, are injected into the current population as parents for crossover and mutation to produce new offspring.

Since the memory pool must be partitioned before each evolutionary generation, an excessively large pool would degrade algorithmic efficiency. Therefore, we cap the memory pool size to match the population size and eliminate individuals from the pool based on an Elimination Weight. To ensure the long-term retention of memories, we introduce the cemetery, which receives individuals with low elimination weights. Given that a marker gene's influence can persist for several generations, eliminating solely on current usefulness may prematurely discard some memories. Therefore, when using the Elimination Weight to decide whether to move an individual to the cemetery, protection is also afforded to those newly added to the memory pool that have not yet exerted their effect. The Elimination Weight is computed as follows:

$$\rho = \frac{UsefulMemoryCount}{\mu(Gen_{Now} - Gen_{Borth})^2} \quad (II.1)$$

Here, *UsefulMemoryCount* denotes the count of effective memories; *Gen<sub>Now</sub>* is the current generation index; *Gen<sub>Borth</sub>* is the generation in which the individual was born,  $\mu$  is the protection coefficient; *Gen<sub>Protect</sub>* is the intended protection span (in generations), during which an individual not selected as useful memory does not experience significant weight decay. The expected protection span *Gen<sub>Protect</sub>* is aligned with the *BufferCount*.  $\mu$  is determined as follows:

$$\mu = \frac{1}{Gen_{Protect}} \quad (II.2)$$

Once an individual in the memory pool is eliminated to the cemetery, its elimination weight ceases to update. If no new individuals are added to the memory pool for *Gen<sub>protect</sub>* consecutive generations, the cemetery selects the individual with the earliest *Gen<sub>Borth</sub>* to re-enter the memory pool, updating its *Gen<sub>Borth</sub>* to the generation immediately preceding its re-entry. To ensure the cemetery can accommodate a sufficient number of marker-gene individuals, its capacity *N* can be set as:

$$N = 2 \left\lceil \frac{Gen}{BufferCount} \right\rceil + 1 \quad (II.3)$$

Here, *Gen* is the target number of generations and *BufferCount* is the Buffer Count threshold.

By establishing both a memory pool and a cemetery, we ensure that marker genes and their entangled counterparts are effectively reintroduced into the population, enabling memory circulation and mitigating memory decay and cyclic relearning.

### III. MGM-RMOEAD on ZDT-1

In this section, we show the actual performance of ZDT-1 in the MGM-RMOEA\D experiment, which will not be analysed more than once here as the difference between the actual performance of ZDT-1 and ZDT-2 is very small. Table I shows the parameters we used in the ZDT-1 benchmark function.

It is obviously that MGM-RMOEA\D performs well in ZDT-1.

### References

- [1] W. Hoeffding, "Probability inequalities for sums of bounded random variables," The collected works of Wassily Hoeffding, pp. 409–426, 1994.
- [2] H. Chernoff, "A measure of asymptotic efficiency for tests of a hypothesis based on the sum of observations," The Annals of Mathematical Statistics, pp. 493–507, 1952.
- [3] M. Freidlin and A. Vent-Tsel', Random perturbations of dynamical systems, Apr 1997, p. 53–94. [Online]. Available: <https://doi.org/10.1090/mmono/161/03>

TABLE I  
Experimental Parameter Settings for ZDT1.

| Parameter                              | MGM-R-MOEA\D      | C-RMOEA\D         |
|----------------------------------------|-------------------|-------------------|
| Population Size ( $N$ )                | 210               | 210               |
| Number of Generations                  | 300               | 300               |
| $X$ Fitness Thread ( $l_X$ )           | 0.0244            | None              |
| $\Delta$ Fitness Thread ( $l_\Delta$ ) | 0.0945            | None              |
| $\delta$ Range ( $\delta_j^i$ )        | $[-0.025, 0.025]$ | $[-0.025, 0.025]$ |
| Number of Decision Variables ( $D$ )   | 10                | 10                |
| Decomposition Method                   | Tchebycheff       | Tchebycheff       |
| Neighborhood Size                      | 20                | 20                |
| Crossover Parameter                    | 0.5               | 0.5               |
| Crossover Probability ( $P_c$ )        | 1.0               | 1.0               |
| Mutation Range                         | $[-0.005, 0.005]$ | $[-0.005, 0.005]$ |
| Mutation Probability ( $P_m$ )         | $1/D$             | $1/D$             |
| Buffer Count                           | 3                 | None              |
| Keep Count                             | 3                 | None              |
| Base weight ( $\omega$ )               | 0.9               | None              |
| Scaling Factor ( $s$ )                 | $10^2$            | None              |

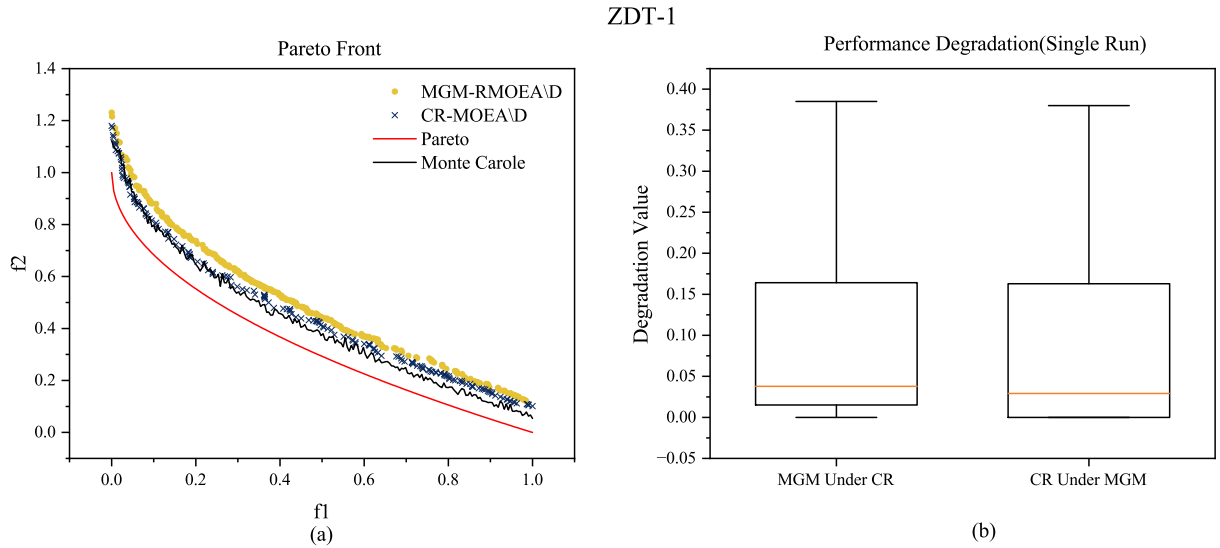

Fig. 1. (a)Performance of MGM-RMOEA\D and CR-MOEA\D on ZDT-1;(b)Box plot of performance degradation about ZDT-1(single run)

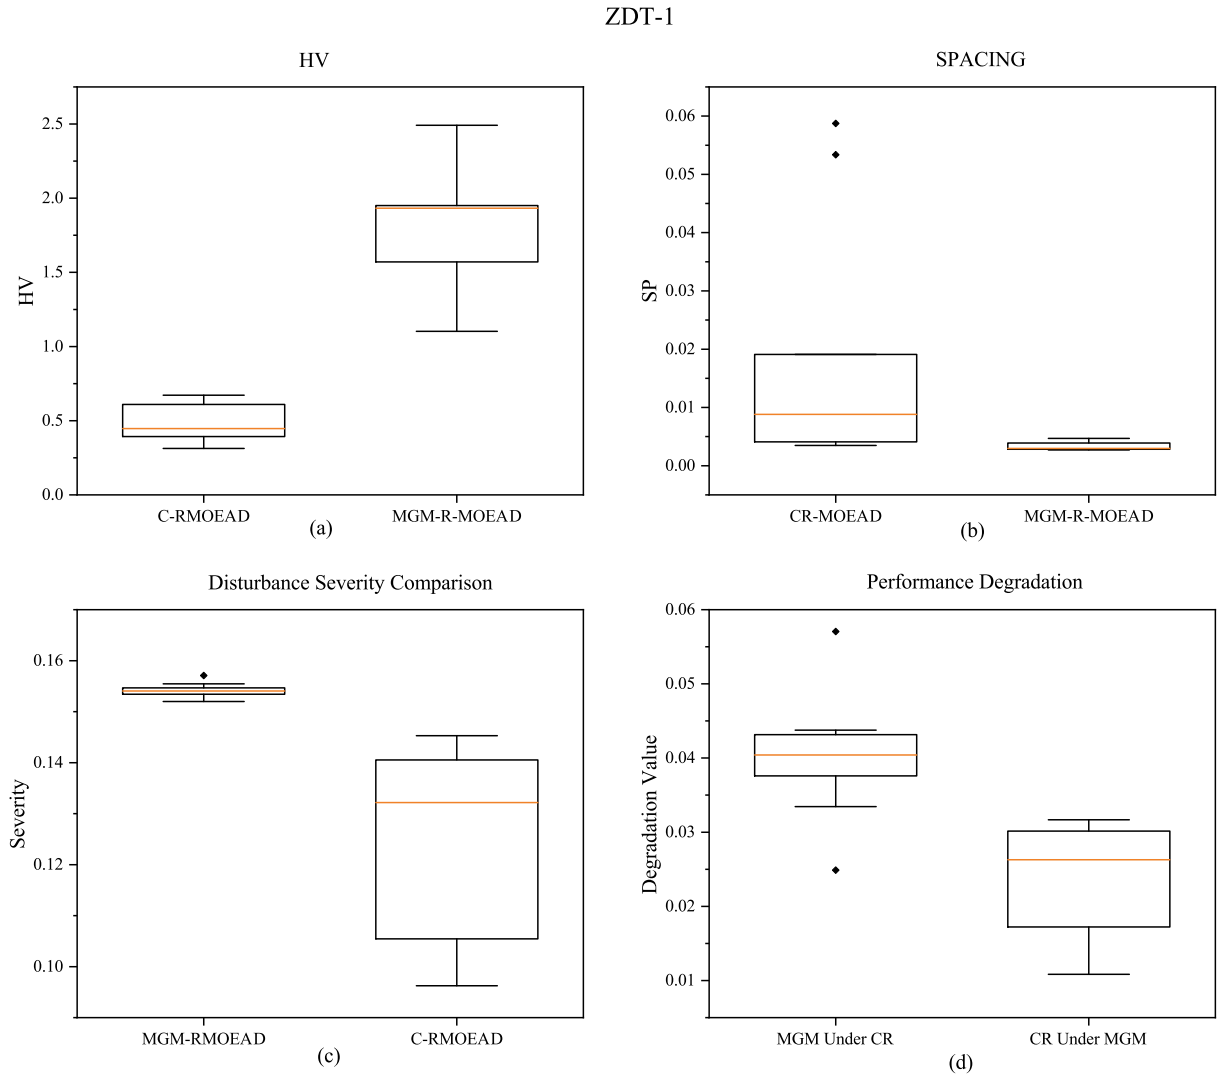

Fig. 2. Comparison of robust multi-objective optimization performance and perturbation characteristics between MGM-RMOEA/D and CR-MOEA/D on the ZDT-1 test function.
